# Supplementary material for: Direct Monocular Odometry Using Points and Lines
Source: arXiv:1703.06380 source file (2017-03-19)
Supplement: Supplementary file 1 [file appendix.tex]

\subsection{Submodular Edge Selection}
Here, we briefly provide the optimality analysis of the edge selection as an extension to Section 
\ref{sec:Optimal boundary detection}. We prove that it is a submodular set selection problem
with matroid constraints \cite{krause2012submodular}.

\subsubsection{Monotonicity}
The score function $F$ in Equation \eqref{eq:edge cost function} is obviously monotonically increasing because
adding more edges, the covering in image horizontal direction will not decrease.

\subsubsection{Submodularity}
We first define the marginal gain of $e$ \textit{wrt.} $S$ as the increase of score $F$ after adding element $e$ into $S$, namely
$$\bigtriangleup(e\mid S) := F(S \cup{ \lbrace e \rbrace}) - F(S)$$

For two sets $S_1 \subset S_2$, edge $e$ may overlap with more edges in $S_2$ and thus reduce the marginal gain compared to
$S_1$, so it satisfies the submodularity condition:
$$ \bigtriangleup(e\mid S_1) \geq  \bigtriangleup(e\mid S_2), \ \forall S_1 \subseteq
S_2 $$
%It is a special case of set covering problem [submodular function maximization, tractability: practical
%approaches.] in 1D.

\subsubsection{Matroid constraint type}
We can remove the edges that are far from CNN boundary before submodular optimization, so we only
consider the second constraint $I_{ovlp}$ in Equation \eqref{eq:edge constraint 2}. Denote all the conflicting edge 
pairs as $ E_i=\lbrace (e_{i1},e_{i2}) \mid O(e_{i1},e_{i2}) \geq \delta_{ovlp} \rbrace, i=1,2,...,k$. 
 For each $E_i$, we form a partition of the ground set $V$ by two disjoint sets 
$P_i=\lbrace E_i,V \setminus E_i \rbrace$ and thus can form a partition matroid constraint $I_{i}^m=\lbrace S\colon | S \cap P_i^1 | \leq 1, | S \cap P_i^2 | \leq n \rbrace$, where $P_i^1$ and $P_i^2$ are two elements of $P_i$.
This is because we can pick at most one element from $E_i$. The union of $k$ such separate matroid constraints 
forms the original constraint $I_{ovlp}=I_{1}^m \cap I_{2}^m... \cap I_{k}^m$.

\subsubsection{Optimality}
From \cite{krause2012submodular}, the greedy algorithm in Equation \eqref{eq:greedy} of 
the submodular optimization with matroid constraints is guaranteed to produce a solution $S$ such that
$F(S) \geq \frac{1}{k+1} \max_{S \subseteq I} F(S)$. It is also important to note that this is only
a worst case bound and in most cases, the quality of solution obtained will be much better than this lower bound.
